# Supplementary material for: Wide Neural Networks as Gaussian Processes: Lessons from Deep Equilibrium Models
Source: arXiv:2310.10767 source file (2023-10-16)
Supplement: Supplementary file 1 [file Extra_exp.tex]

% !TEX root = ../neurips_2023.tex

\section{Additional Experimental Results}\label{app: extra_exp}
Code is made at https://github.com/deqg/deq.git.

\subsection*{Distribution of the output distribution}
\begin{figure}[h]
    \centering
    \includegraphics[width=0.3\linewidth]{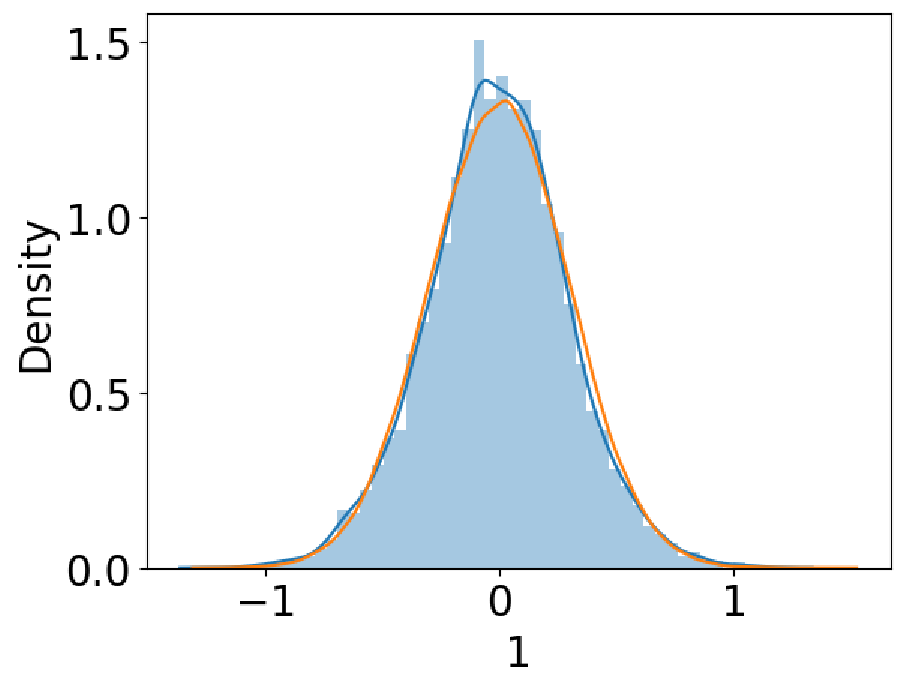}
    \includegraphics[width=0.3\linewidth]{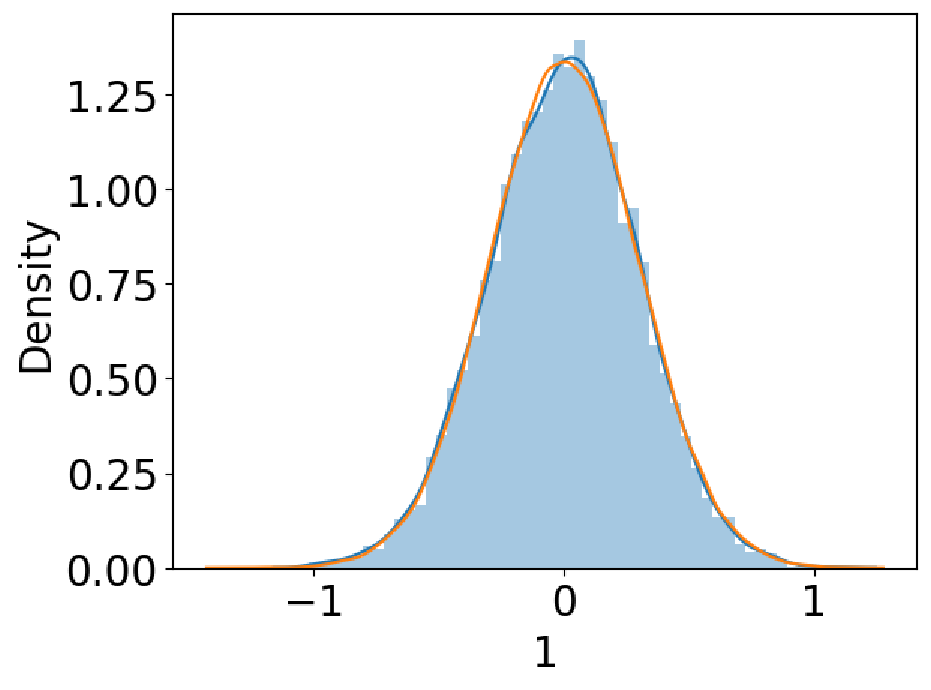}
    \includegraphics[width=0.3\linewidth]{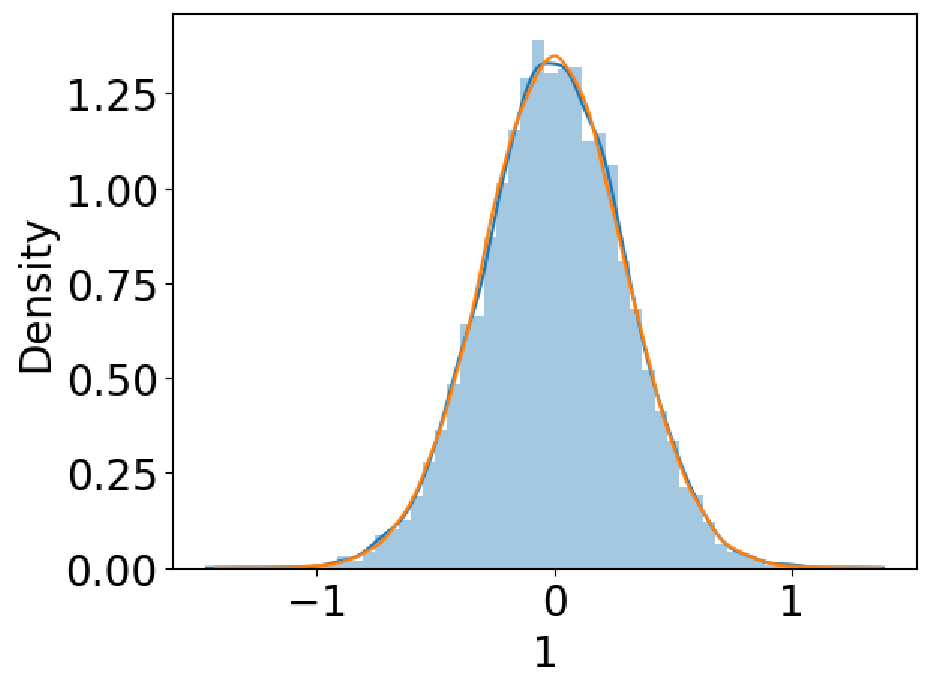}
    \includegraphics[width=0.3\linewidth]{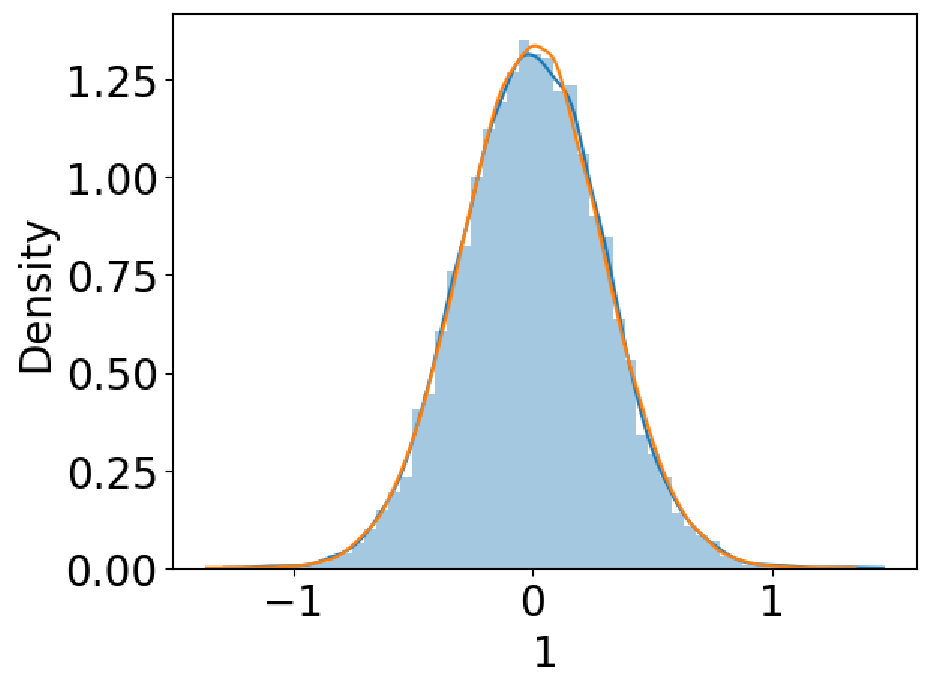}
    \includegraphics[width=0.3\linewidth]{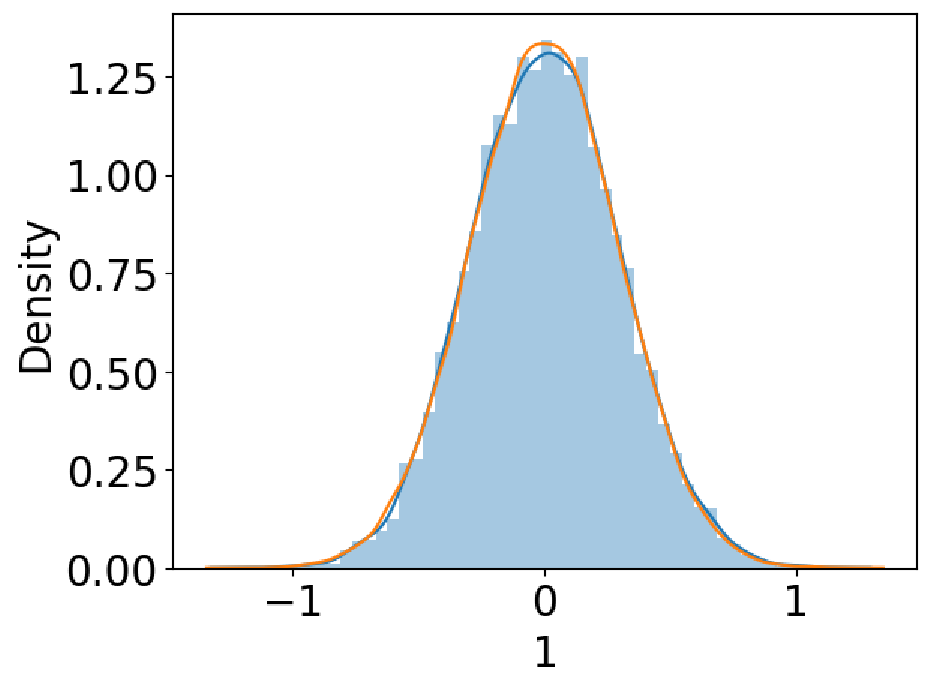}
    \caption{Histplot of the distribution of $h^L$ for five neural networks with widths 10, 50, 100, 500, 1000 (left to right); KS statistics: $0.0154,0.0080, 0.0054, 0.0065,0.0068$, pvalue: $0.0173, 0.5395, 0.9331,0.7924,0.7446$.}
    \label{supp_fig:gaussian}
\end{figure}

\subsection*{Results for different activation function relu}
 
\begin{figure}[h]
	\centering
        \includegraphics[height=0.26\linewidth]{images/relu/fix.eps}
        \includegraphics[height=0.26\linewidth]{images/relu/pairplot.eps}
        \includegraphics[height=0.26\linewidth]{images/relu/gaussian_1000.eps}
	\caption{Plot of Figure \ref{fig:1} with activation function relu}
 \end{figure}

\begin{figure}
	\centering
        \includegraphics[height=0.24\linewidth]{images/relu/gaussian.eps}
        \includegraphics[height=0.24\linewidth]{images/relu/cov1.eps}
        \includegraphics[height=0.24\linewidth]{images/relu/cov2.eps}
	\caption{Plot of Figure \ref{fig:kernel} with activation function relu}
\end{figure}

\begin{figure}
    \centering
    \begin{tabular}{cccc}
            \includegraphics[width=0.22\textwidth]{images/relu/cov_width.eps}
 &     \includegraphics[width=0.22\textwidth] {images/relu/cov_wdith1.eps} &
             \includegraphics[width=0.22\textwidth]{images/relu/cov_depth.eps}
& \includegraphics[width=0.22\textwidth]{images/relu/cov_depth1.eps}
    \end{tabular}
    \caption{Plot of Figure \ref{fig:cov_width_depth} with activation function relu}
\end{figure}
\begin{figure}
    \centering
        \begin{tabular}{cccc}
    \includegraphics[width=0.22\linewidth]{images/relu/lam.eps} &    \includegraphics[width=0.22\linewidth]{images/relu/lamlam.eps}& \includegraphics[width=0.22\linewidth]{images/relu/lam_sim_width.eps}
&   \includegraphics[width=0.22\linewidth]{images/relu/lam_eig_sigma.eps}
    \end{tabular}
    \caption{Plot of Figure \ref{fig:eig} with activation function relu}
\end{figure}

\begin{figure}[h]
    \centering
    \includegraphics[width=0.22\linewidth]{images/relu/gaussian_50.eps}
    \includegraphics[width=0.22\linewidth]{images/relu/gaussian_100.eps}
    \includegraphics[width=0.22\linewidth]{images/relu/gaussian_500.eps}
    \includegraphics[width=0.22\linewidth]{images/relu/gaussian_1000.eps}
    \caption{Plot of Figure \ref{supp_fig:gaussian} with activation function relu; KS statistics: $0.1217,0.0137, 0.0127, 0.0070,0.0056$, pvalue: $ 1.88\times 10^{-129}, 0.0456,0.0774,0.7138,0.9057$.}

\end{figure}
